# Supplementary material for: Many-Body-Expansion Based on Variational Quantum Eigensolver and Deflation for Dynamical Correlation
Source: arXiv:2310.03954 source file (2023-10-06)
Supplement: Supplementary file 1 [file SI.pdf]

# Supporting Information for “Many-Body-Expansion Based on Variational Quantum Eigensolver and Deflation for Dynamical Correlation”

Xu Enhua,<sup>†</sup> Yuma Shimomoto,<sup>†</sup> Seiichiro L. Ten-no,<sup>†</sup> and Takashi Tsuchimochi<sup>\*,†</sup>

<sup>†</sup>*Graduate School of System Informatics, Kobe University, 1-1 Rokkodai-cho, Nada-ku,  
Kobe, Hyogo 657-8501 Japan*

<sup>‡</sup>*Japan Science and Technology Agency (JST), Precursory Research for Embryonic Science  
and Technology (PRESTO), 4-1-8 Honcho Kawaguchi, Saitama 332-0012 Japan*

E-mail: tsuchimochi@gmail.com

Table S1: MAE and NPE with respect to MRCI+Q in the PES of the bond dissociation process of the ground state of H<sub>2</sub>O. The aug-cc-pVDZ basis set is employed and all the data are in mH.

|                         | MAE  | NPE  |
|-------------------------|------|------|
| MBE(2)-UCCSD            | 14.3 | 21.9 |
| MBE(3)-UCCSD            | 15.0 | 19.9 |
| MBE(2)-UCCGSD/UCCpGSD   | 9.7  | 15.9 |
| MBE(3)-UCCGSD/UCCpGSD   | 8.6  | 14.8 |
| MBE(2)-ooUCCGSD/UCCpGSD | 1.3  | 2.0  |
| MBE(3)-ooUCCGSD/UCCpGSD | 0.8  | 0.7  |

Figure S1: Absolute and relative (with respect to MRCI+Q) energies of different approaches in the bond dissociation process of the ground state of  $\text{H}_2\text{O}$  with the aug-cc-pVDZ basis set.

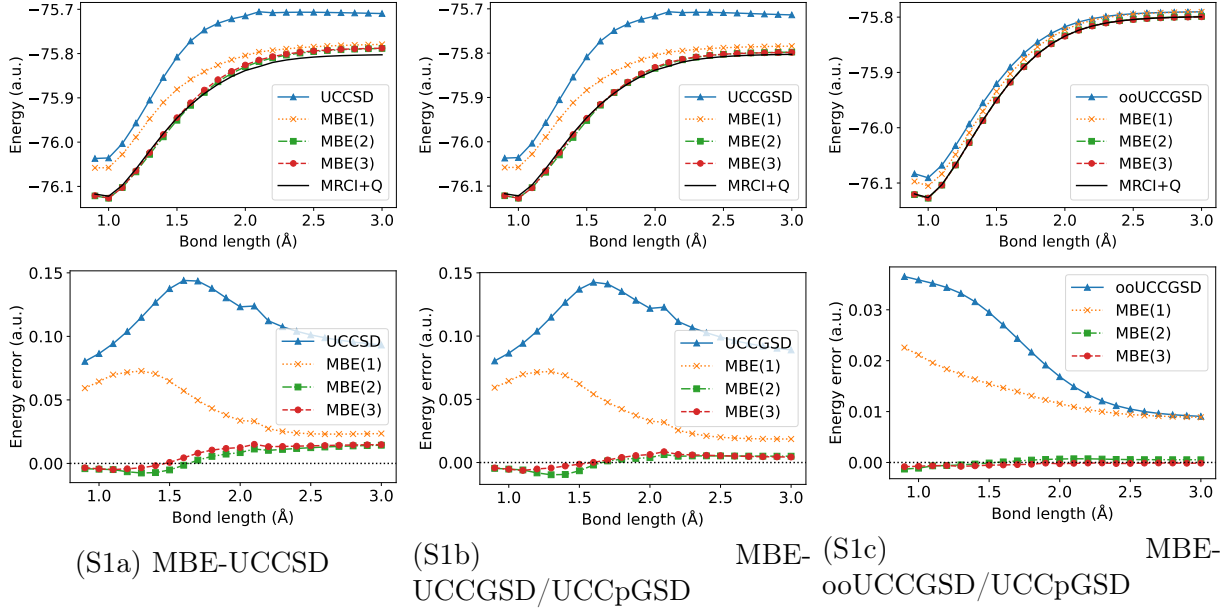

Figure S2: Absolute and relative (with respect to MRCI+Q) energies of different approaches in the bond dissociation of the ground state of  $\text{N}_2$  with the aug-cc-pVDZ basis set.

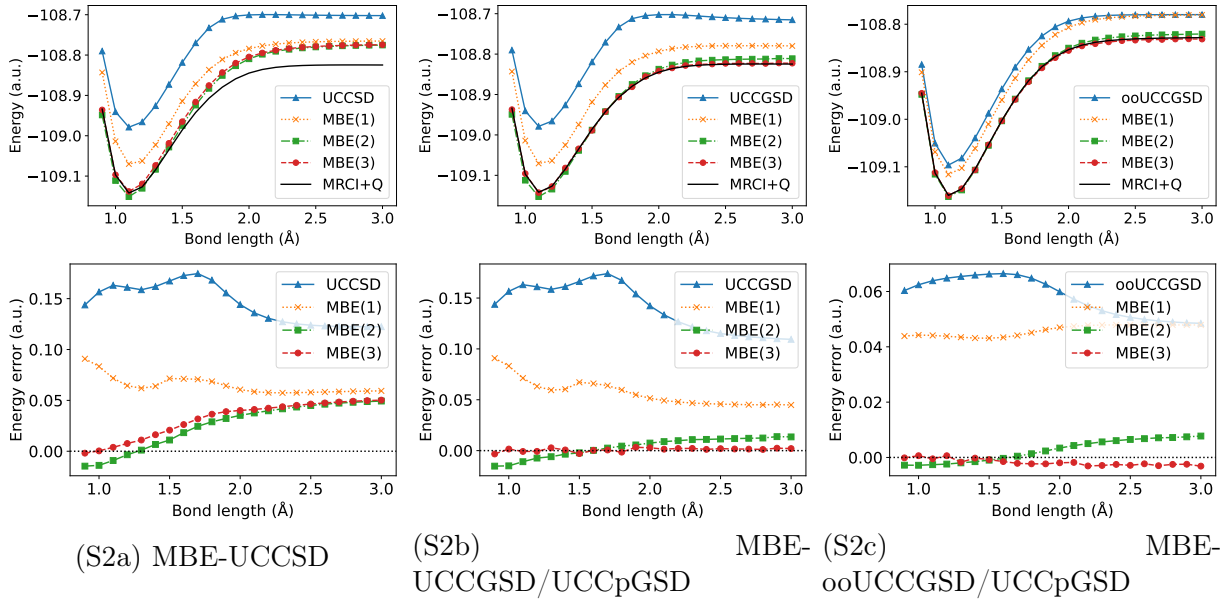

Table S2: MAE and NPE with respect to MRCI+Q in the PES of the bond dissociation of the ground state of N<sub>2</sub>. The aug-cc-pVDZ basis set is employed and all the data are in mH

|                         | MAE  | NPE  |
|-------------------------|------|------|
| MBE(2)-UCCSD            | 49.3 | 64.0 |
| MBE(3)-UCCSD            | 50.3 | 52.1 |
| MBE(2)-UCCGSD/UCCpGSD   | 15.3 | 29.0 |
| MBE(3)-UCCGSD/UCCpGSD   | 3.3  | 6.5  |
| MBE(2)-ooUCCGSD/UCCpGSD | 7.7  | 10.6 |
| MBE(3)-ooUCCGSD/UCCpGSD | 3.1  | 3.8  |

Table S3: MBE energies calculated by different approaches for the ground state ( $1^1\Sigma^+$ ) and two excited states ( $1^3\Sigma^+$ ,  $2^1\Sigma^+$ ) of LiH with the cc-PVDZ basis set. There is no core orbital frozen and the lowest four orbitals are optimized as the active space. The ground state energies are in a.u. and the vertical excited energies are in eV.

| State              | $1^1\Sigma^+$ | $1^3\Sigma^+$ | $2^1\Sigma^+$ |
|--------------------|---------------|---------------|---------------|
| MBE-UCCSD          |               |               |               |
| Ref                | -7.932325     | 0.02          | 1.67          |
| MBE(1)             | -7.932508     | 0.03          | 1.64          |
| MBE(2)             | -7.932558     | 0.03          | 1.64          |
| MBE(3)             | -7.932560     | 0.03          | 1.64          |
| MBE-UCCGSD/UCCpGSD |               |               |               |
| Ref                | -7.932329     | 0.02          | 1.67          |
| MBE(1)             | -7.932578     | 0.03          | 1.64          |
| MBE(2)             | -7.932671     | 0.03          | 1.64          |
| MBE(3)             | -7.932672     | 0.03          | 1.64          |
| MBE-FCI            |               |               |               |
| Ref                | -7.932329     | 0.02          | 1.67          |
| MBE(1)             | -7.932578     | 0.03          | 1.64          |
| MBE(2)             | -7.932671     | 0.03          | 1.64          |
| MBE(3)             | -7.932672     | 0.03          | 1.64          |
| FCI                | -7.933503     | 0.03          | 1.64          |

Table S4: MBE energies calculated by different approaches for the ground state ( $1^1\Sigma^+$ ) and two excited states ( $1^1\Delta$ ,  $2^1\Sigma^+$ ) of CH+ with the aug-cc-pVDZ basis set. The 1s core orbital is frozen and the next lowest five orbitals are optimized as the active space. The ground state energies are in a.u. and the vertical excited energies are in eV.

| State              | $1^1\Sigma^+$ | $1^1\Delta$ | $2^1\Sigma^+$ |
|--------------------|---------------|-------------|---------------|
| MBE-UCCSD          |               |             |               |
| Ref                | -37.954326    | 7.28        | 9.00          |
| MBE(1)             | -37.992373    | 7.93        | 9.07          |
| MBE(2)             | -38.003170    | 4.05        | 9.10          |
| MBE(3)             | -38.002597    | 38.29       | 9.28          |
| MBE-UCCGSD/UCCpGSD |               |             |               |
| Ref                | -37.954315    | 7.27        | 8.66          |
| MBE(1)             | -37.992905    | 6.86        | 8.58          |
| MBE(2)             | -38.004947    | 6.83        | 8.42          |
| MBE(3)             | -38.004443    | 6.85        | 8.40          |
| MBE-FCI            |               |             |               |
| Ref                | -37.954315    | 7.27        | 8.66          |
| MBE(1)             | -37.992905    | 6.86        | 8.58          |
| MBE(2)             | -38.004948    | 6.83        | 8.42          |
| MBE(3)             | -38.004445    | 6.86        | 8.40          |
| FCI                | -38.004247    | 6.87        | 8.42          |

Table S5: MBE energies calculated by different approaches for the ground state ( $1^1A_1$ ) and two excited states ( $1^3A_1$  and  $2^1A_1$ ) of water with the aug-cc-pVDZ basis set. The 1s core orbital is frozen and the next lowest six orbitals are optimized as the active space. The ground state energies are in a.u. The vertical excited energies are in eV.

| State              | $1^1A_1$   | $1^3A_1$ | $2^1A_1$ |
|--------------------|------------|----------|----------|
| MBE-UCCGSD/UCCpGSD |            |          |          |
| Ref                | -76.040609 | 8.47     | 9.03     |
| MBE(1)             | -76.161798 | 9.64     | 9.98     |
| MBE(2)             | -76.288834 | 9.84     | 10.25    |
| MBE(3)             | -76.271080 | 9.38     | 9.89     |
| MBE-FCI            |            |          |          |
| Ref                | -76.040609 | 8.47     | 9.03     |
| MBE(1)             | -76.161803 | 9.64     | 9.98     |
| MBE(2)             | -76.288923 | 9.83     | 10.25    |
| MBE(3)             | -76.273263 | 9.35     | 9.82     |
| exFCI              |            | 9.49     | 9.94     |
